# Supplementary material for: Deep Chain HDRI: Reconstructing a High Dynamic Range Image from a Single Low Dynamic Range Image
Source: arXiv:1801.06277 ancillary file (2018-01-19)
Supplement: Supplementary file 1 [file egpaper_final_opt.pdf]

# Supplementary Material
## Deep Chain HDRI: Reconstructing a High Dynamic Range Image from a Single Low Dynamic Range Image

Siyeong Lee Gwon Hwan An Suk-Ju Kang
Sogang University
Seoul, Republic of Korea
{siyeong, ghan, sjkang}@sogang.ac.kr

### Abstract

*This supplementary file presents 1. validity of the chain structure neural network, 2. new activation function MPReLU for the Deep Chain HDRI method, and 3. experimental results using our datasets.*

## 1. Validity of the chain structure neural network

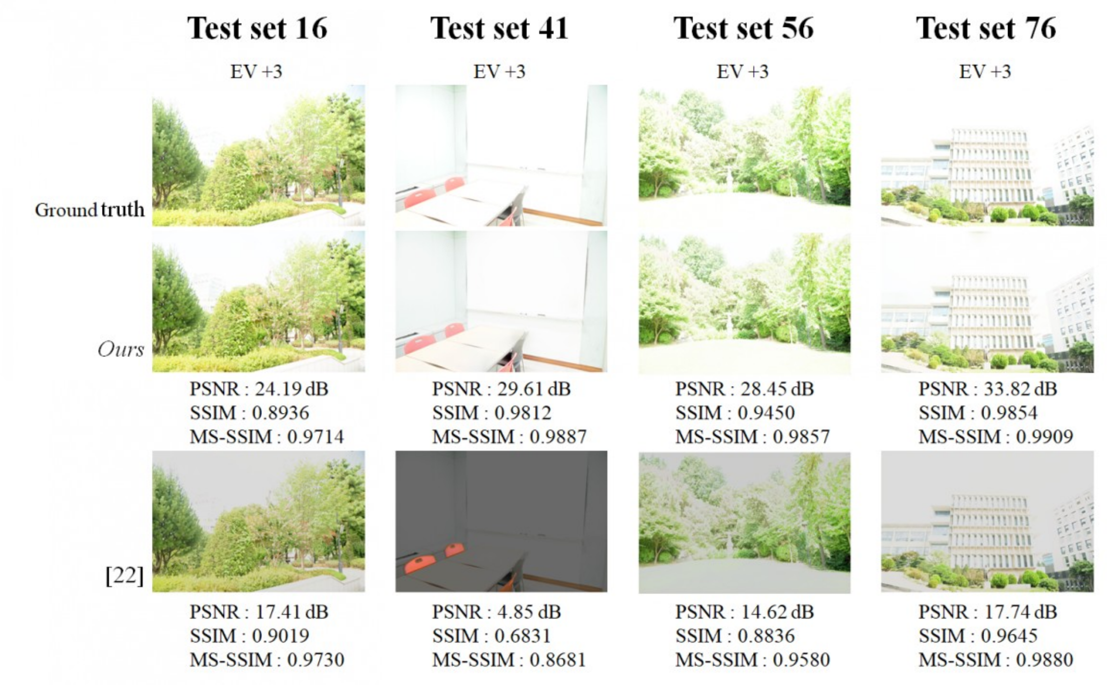


Figure 1. Comparison of the proposed method with a relatively shallow network that is skip-connected between three convolution layers and three deconvolution layers [22] for the problem of inferring the relationship between EV 0 and EV +3.

## 2. New activation function MPReLU for the Deep Chain HDRI method

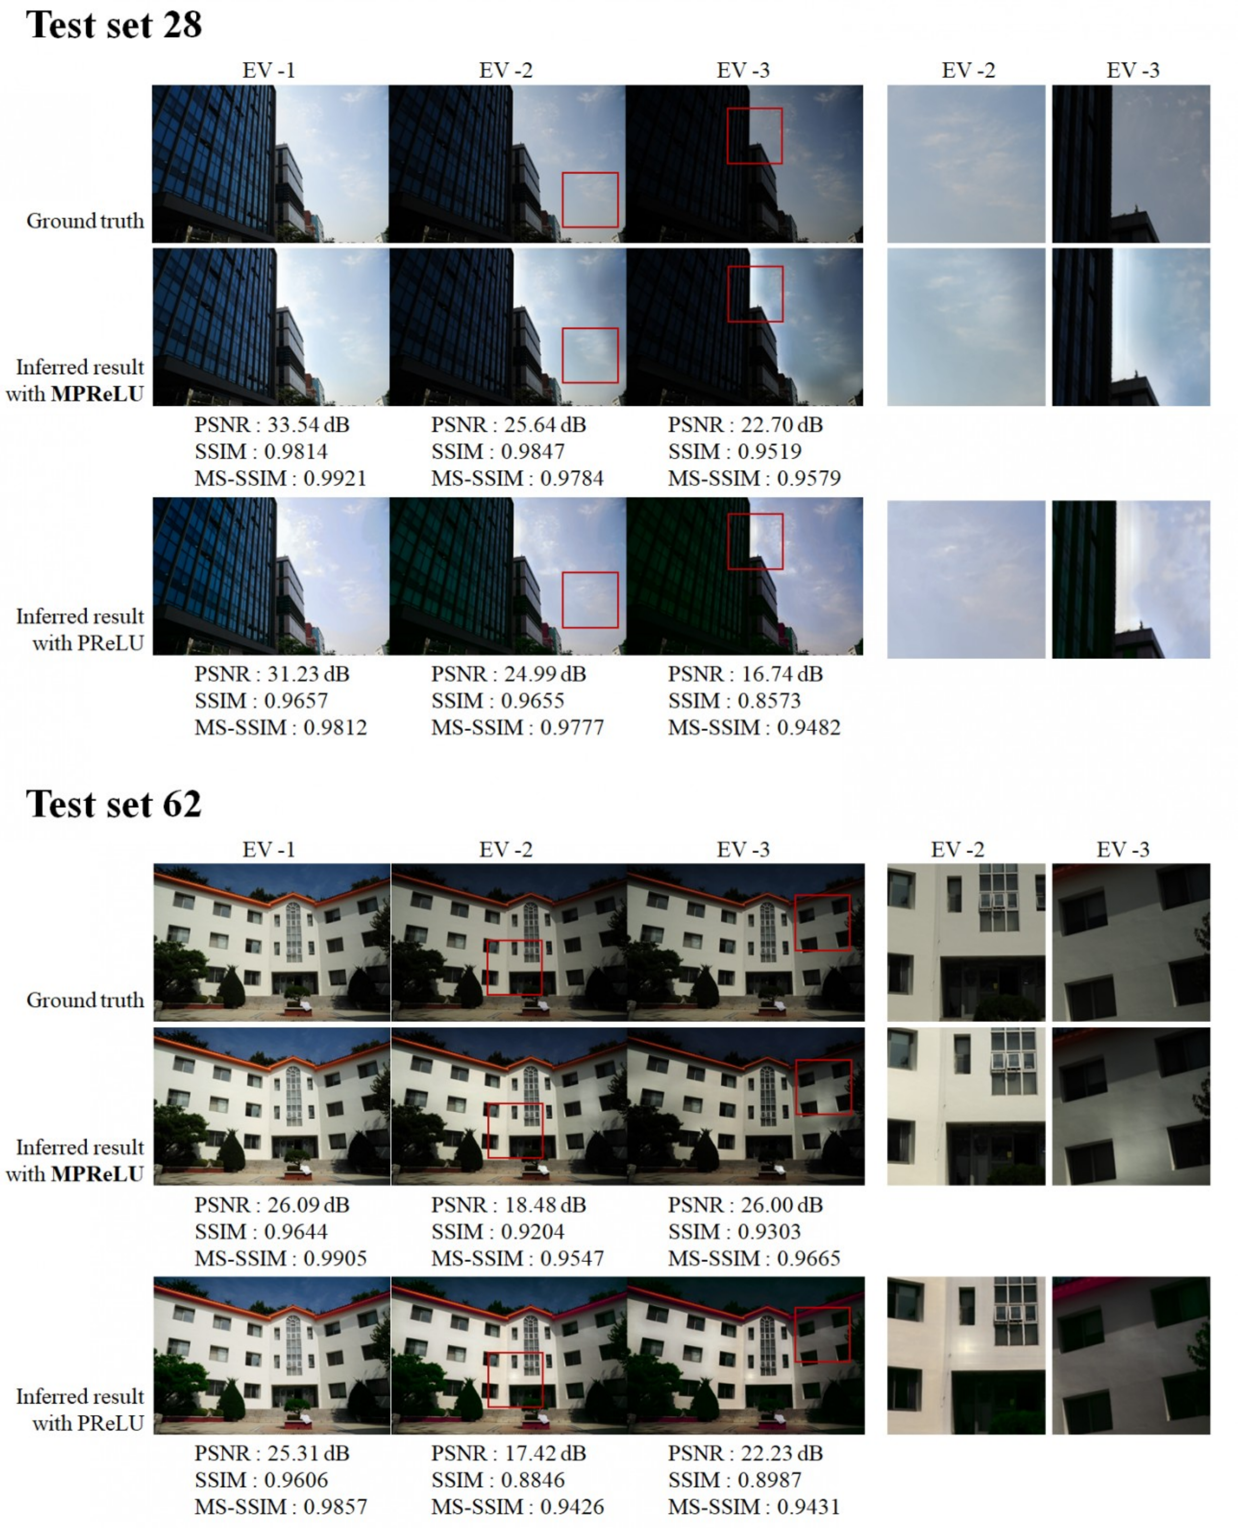


Figure 2. Comparison of the proposed MPReLU with PReLU for problems with a lower exposure (darker) images.

# 3. Experimental results

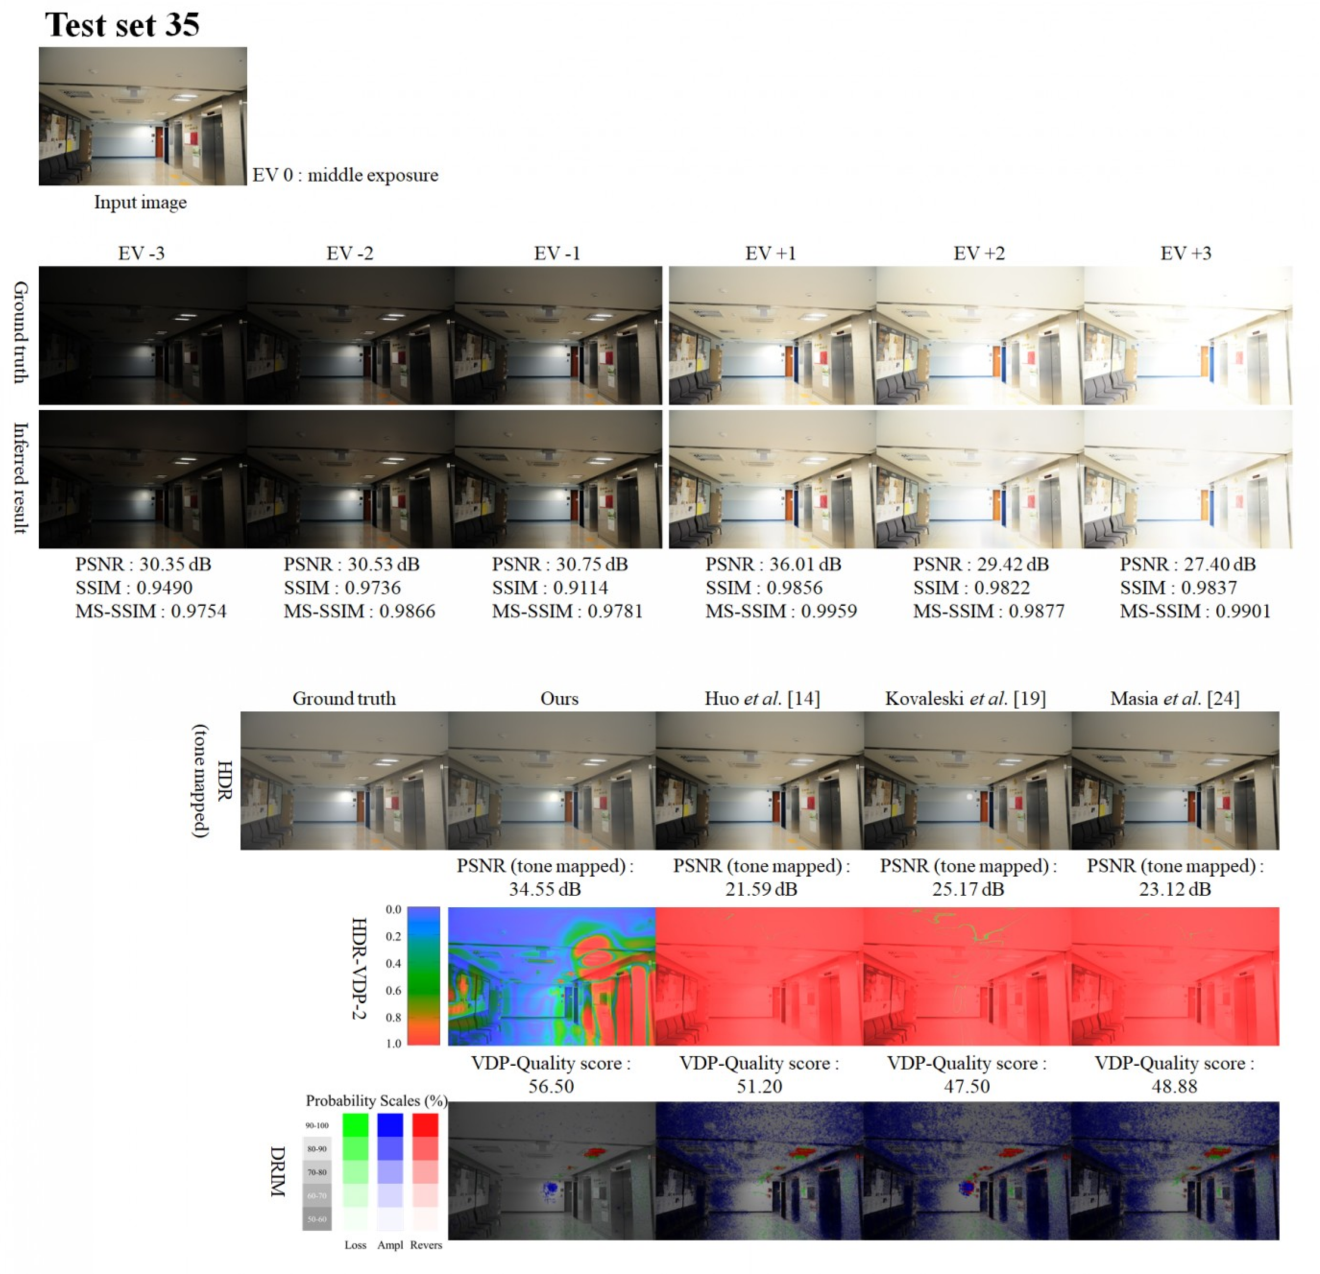


Figure 3. Comparison of the ground truth LDR image stack and inferred LDR image stack (top) & comparison of the ground truth HDR images inferred by the proposed and conventional method (bottom) for test set #35.

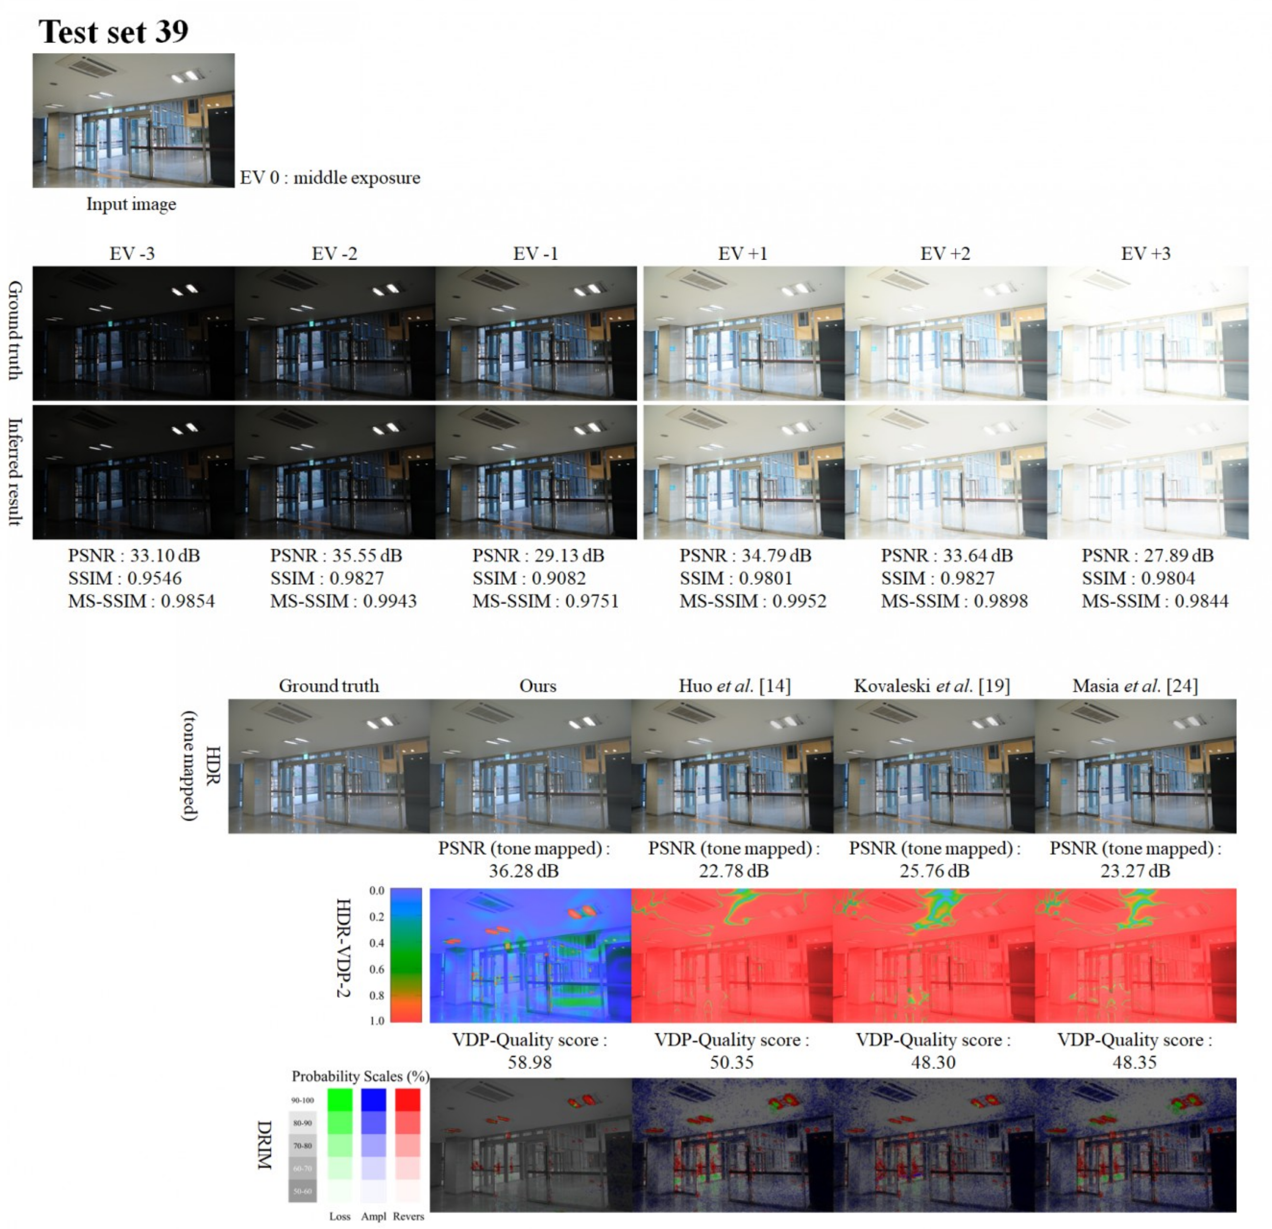


Figure 4. Comparison of the ground truth LDR image stack and inferred LDR image stack (top) & comparison of the ground truth HDR images inferred by the proposed and conventional method (bottom) for test set #39.

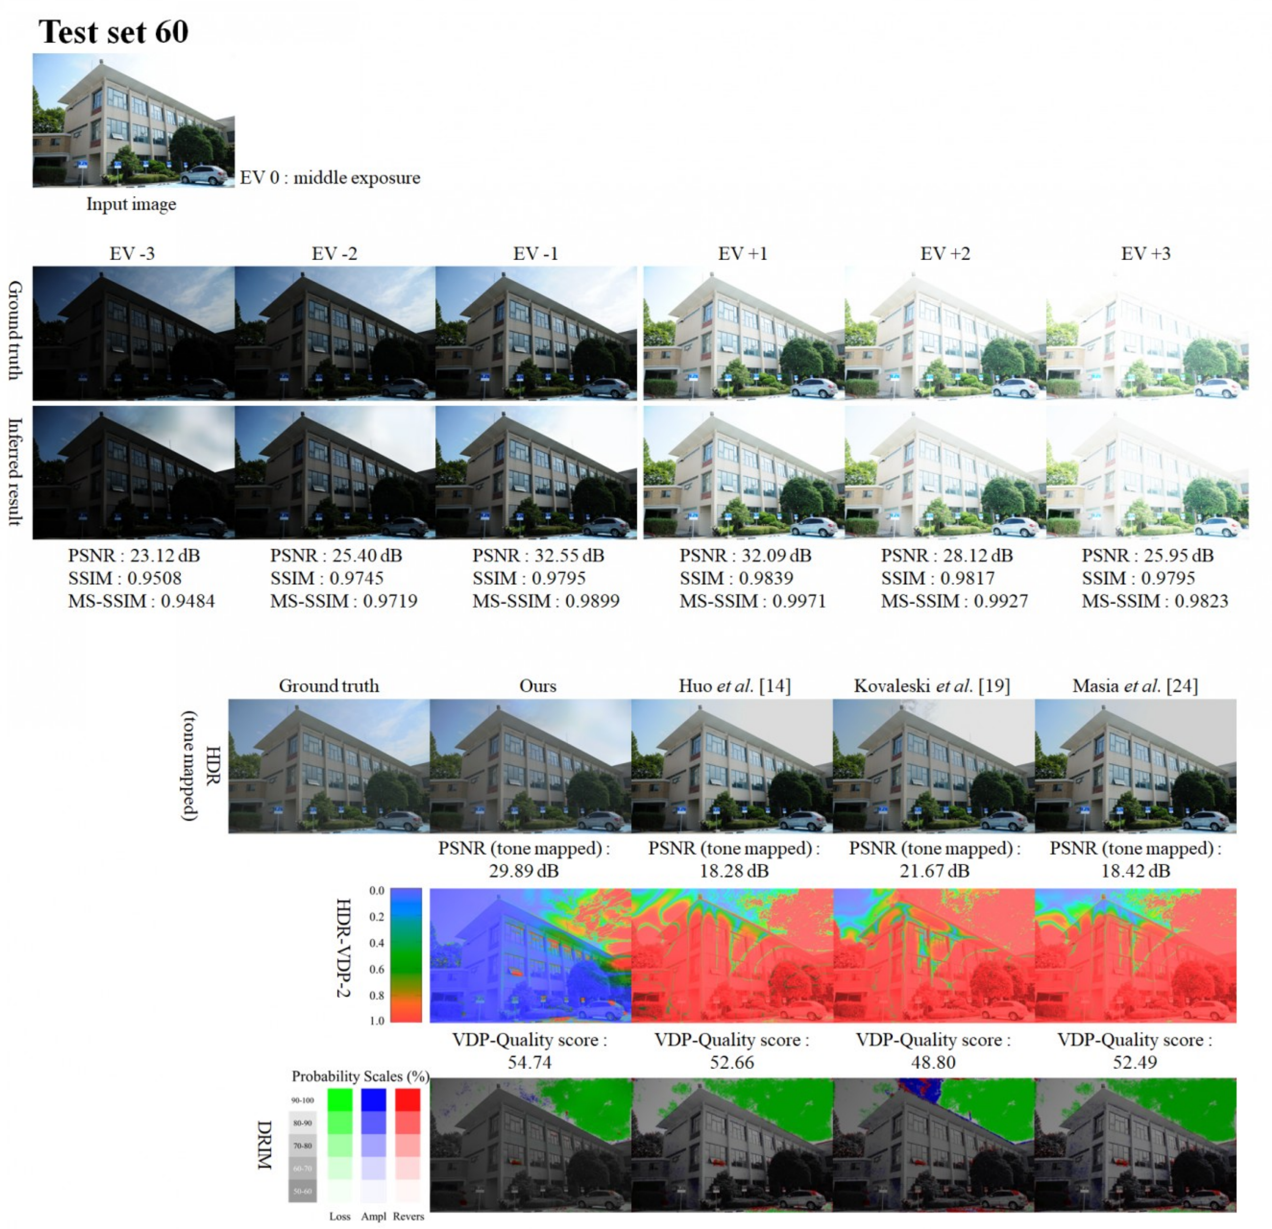


Figure 5. Comparison of the ground truth LDR image stack and inferred LDR image stack (top) & comparison of the ground truth HDR images inferred by the proposed and conventional method (bottom) for test set #60.

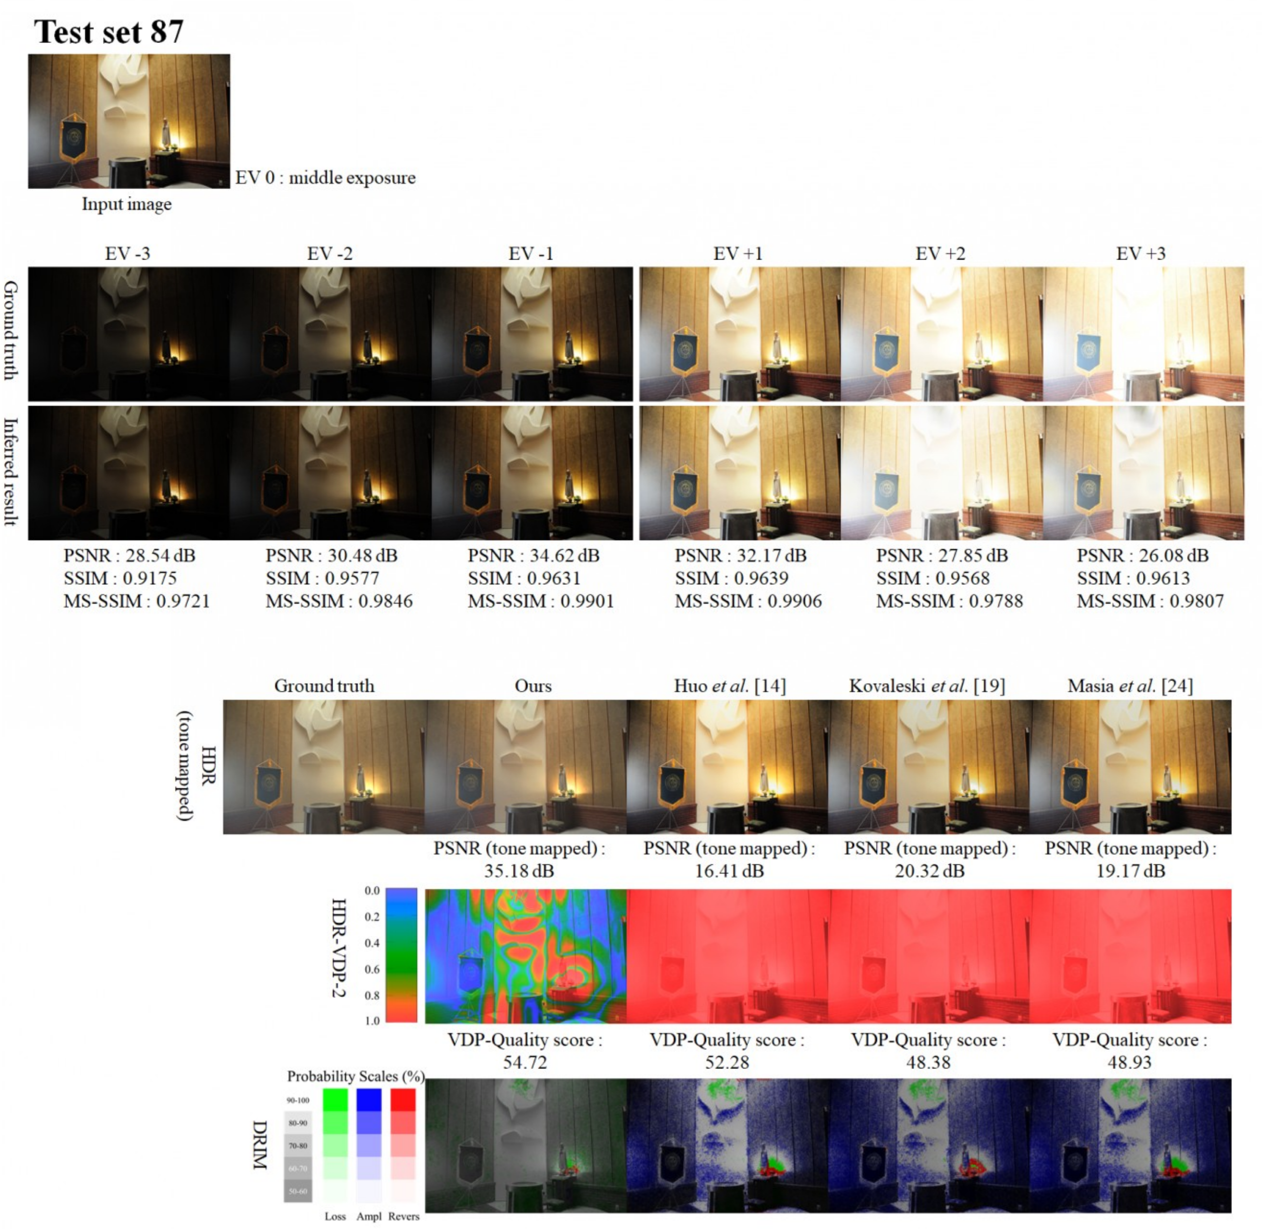


Figure 6. Comparison of the ground truth LDR image stack and inferred LDR image stack (top) & comparison of the ground truth HDR images inferred by the proposed and conventional method (bottom) for test set #87.

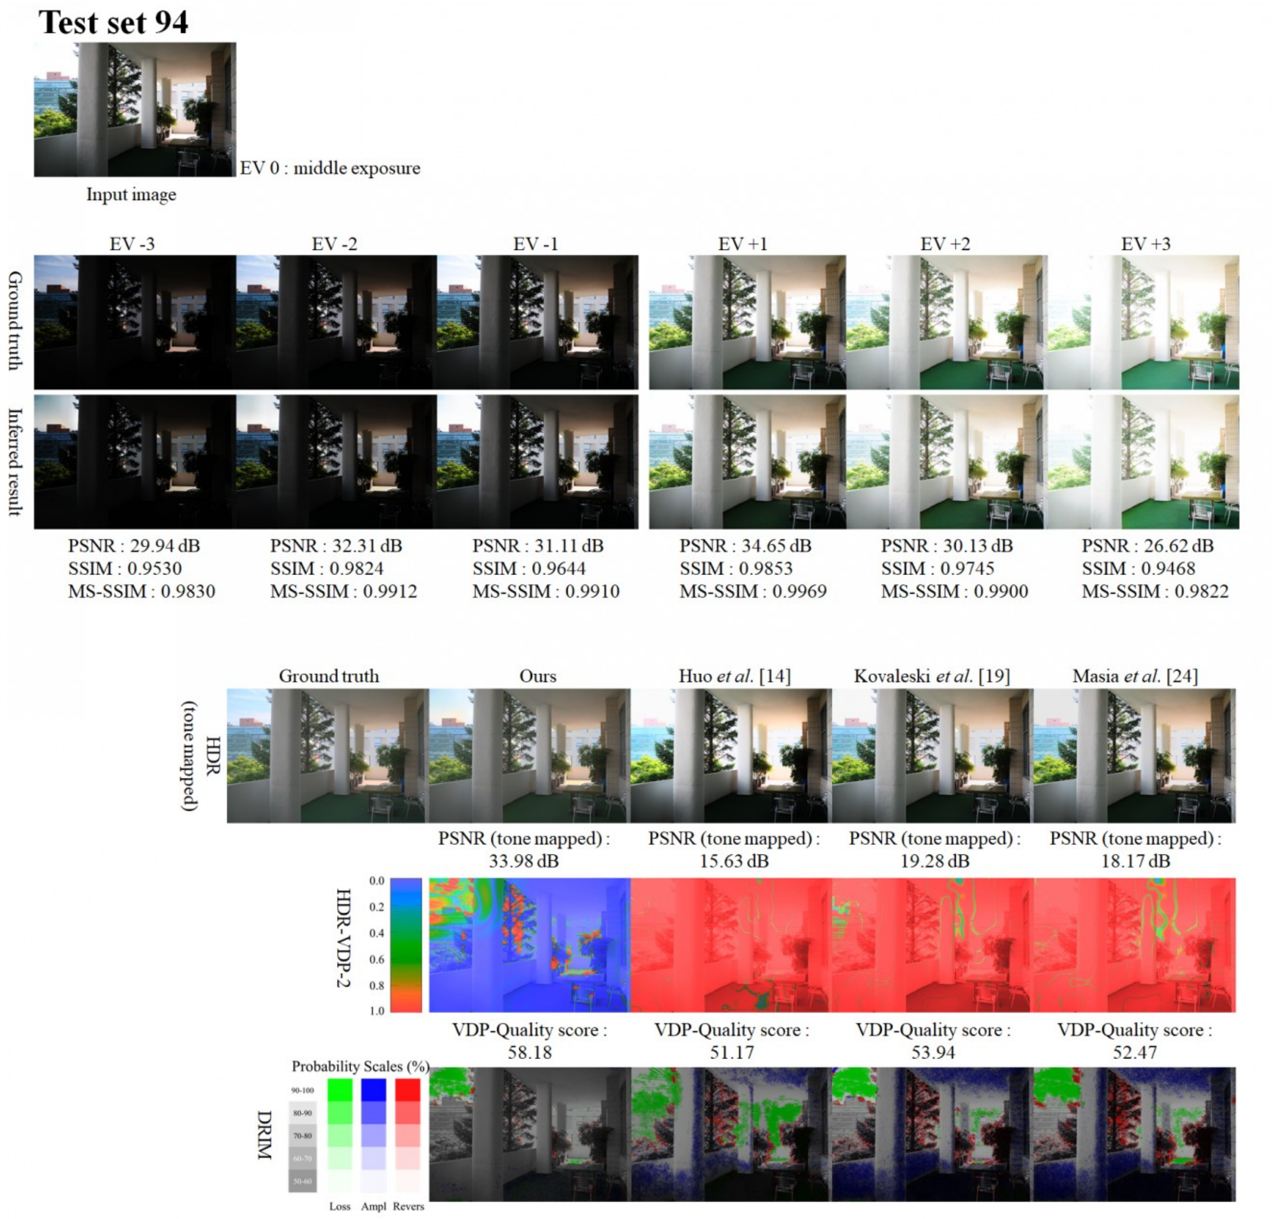


Figure 7. Comparison of the ground truth LDR image stack and inferred LDR image stack (top) & comparison of the ground truth HDR images inferred by the proposed and conventional method (bottom) for test set #94.

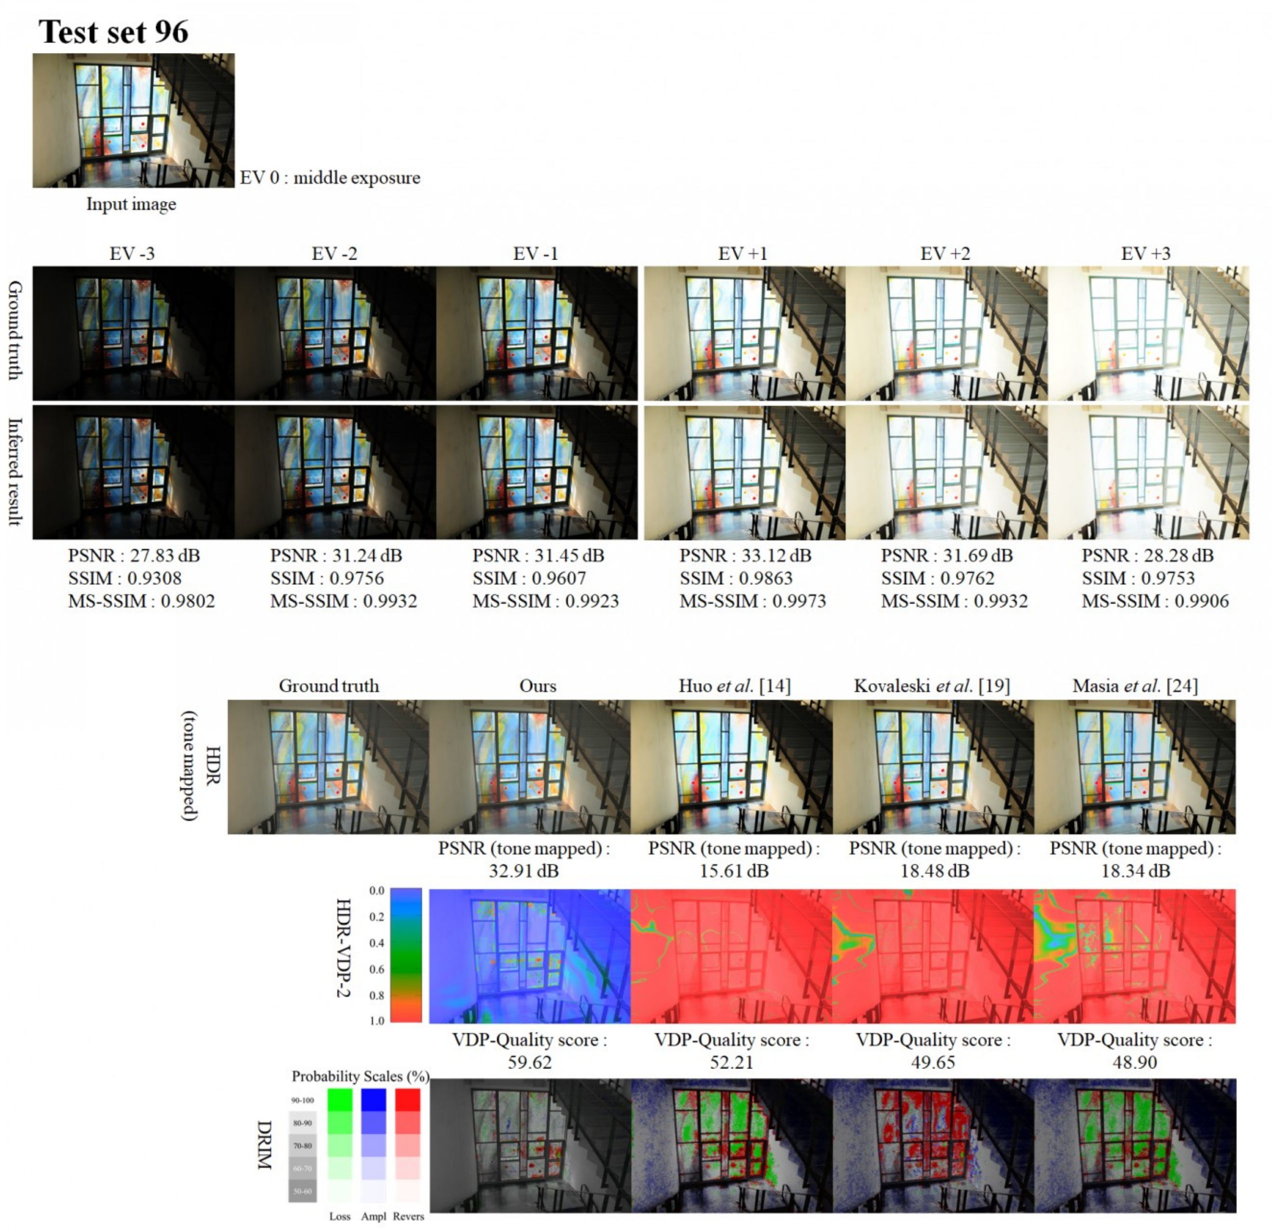


Figure 8. Comparison of the ground truth LDR image stack and inferred LDR image stack (top) & comparison of the ground truth HDR images inferred by the proposed and conventional method (bottom) for test set #96.
